# Supplementary material for: The Hidden cost of the Edge: A Performance Comparison of Edge and Cloud Latencies
Source: arXiv:2104.14050 source file (2021-04-29)
Supplement: Supplementary file 1 [file appendix.tex]

% Please add the following required packages to your document preamble:
% \usepackage[table,xcdraw]{xcolor}
% If you use beamer only pass "xcolor=table" option, i.e. \documentclass[xcolor=table]{beamer}
\section{Appendix}

\subsection{Artifact Evaluation}
We present the toolset used in this research as a general and extensible performance benchmarking framework for real-world edge/cloud environments. Our framework, which is built based on a variety of mature open-source technologies, enables automatic infrastructure provisioning, workload deployment, benchmark execution, and metrics collection.

Our performance benchmark uses a client/server architecture: the client side is one node running the load generator, while the server side is a cluster which consists of one load-balancer node and multiple worker nodes. We use Gatling~\footnote{https://gatling.io/}, an open-source load testing tool, as the load generator. We implemented two load patterns using Gatling for the evaluation in this paper: constant rate Poisson processes, and emulations using  Azure Functions Traces~\footnote{https://github.com/Azure/AzurePublicDataset}. Gatling also support other distributions such as evenly distributed requests or requests with ramp-up arrival rate. More complex patterns can also be implemented by either 1) describing the simulation procedures using Scala scripts, or 2) recording user behaviors using a bundled recorder and replaying the recorded scenarios during benchmark experiments. 

On the server cluster side, each worker node runs an instance of the deep learning REST API server based on Keras and TensorFlow~\footnote{Our system deployment is similar to: https://blog.keras.io/building-a-simple-keras-deep-learning-rest-api.html}. We use docker as the server runtime to make it easier to change the server application to any other application. For the the load-balancer we use HAProxy running in multi-thread mode to handle high throughput. After receiving requests from the workload generator, HAProxy will distribute the requests among available worker nodes using the lead connection load balancing algorithm in order to maximize resource multiplexing.

For users who want to run the benchmark in a public cloud, we also provide automation scripts based on Terraform for describing and provisioning the desired infrastructure. Although we currently only implement the scripts for AWS EC2, Terraform has support for most major cloud providers, such as Microsoft Azure and Google Cloud, so the scripts can be easily modified to work with other providers. The configurations of all the nodes used in the experiment, including regions/availability zones, instance types, SSH key pair, and the number of worker nodes, can be specified in the scripts. Once the scripts have been properly configured, a user can just use one single command to set up or tear down the testing infrastructure, as demonstrated in the sample workflow below.

Once the testing infrastructure is set up, our framework provide a set of Ansible playbooks for automating the deployment of the performance benchmark. All the aforementioned software components used for the benchmarking experiments will be installed and configured using Ansible. Users can change these playbooks to modify the software environment to their needs. For example, to change the server application running on the worker nodes, a user only need to change a few parameters in the \texttt{docker\_image} and \texttt{docker\_container} modules in the worker setup playbook. In addition, the experiment execution and data collection are also implemented as playbooks to improve efficiency. For instance, users can run multiple benchmarking scenarios at once to fully explore the performance characteristics, or collect CPU utilization data from all the worker nodes in parallel.

The workflow of a typical run of the benchmarking framework looks like follows:

\begin{lstlisting}[basicstyle=\footnotesize]
terraform apply -var load-generator-region=us-east-2 \
                -var cluster-region=ca-central-1 \
                -var worker-count=10 -auto-approve
                
(cd ansible && \
    ansible-playbook ping.yml && \
    ansible-playbook setup.yml && \
    ansible-playbook experiment.yml)

terraform destroy -var load-generator-region=us-east-2 \
                  -var cluster-region=ca-central-1 \
                  -var worker-count=10 -auto-approve
\end{lstlisting}       

Thanks to Gatling, after the benchmark experiment is finished an HTML report will be generated for each simulation with many statistics and beautiful visualizations, such as the response time distribution, response time percentiles over time, number of requests per second, etc. These reports can help users develop quick insights into the system performance and possible bottlenecks. Our framework will also collect and download more fine-grained data including 

\begin{enumerate}
    \item The RTT between the load generator and the load balancer, which is measured using the \texttt{ping} command.  
    
    \item The start time and completion time of each request, which is observed on the load generator node.
    
    \item The service time of each request, which is observed on each worker node. We record the system time before and after the processing of each request, then attach the elapsed time as a filed in the json response. We will then use Gatling to parse the json responses to extract the service times, and save them into a separate file. Similarly, any information contained in the response can be parsed and saved.
    
    \item The CPU utilization of each worker node throughout the duration of the experiment. This is collected by running the \texttt{mpstat} command. Our automation script will start \texttt{mpstat} before the benchmark starts and let it run at 1 second intervals. The command output will be saved to a file and downloaded later after the benchmark completes.
\end{enumerate}
These fine-grained data can be processed to generate more detailed performance metrics if needed.

Our performance benchmarking framework is released as an open-source artifact, available at \textit{URL blinded for review}.
